# Supplementary material for: Thermostat: A Large Collection of NLP Model Explanations and Analysis Tools
Source: arXiv:2108.13961 source file (2021-08-31)
Supplement: Supplementary file 1 [file appendix.tex]

\section*{Appendix}
\label{sec:Appendix}

\subsection*{Implementation details}

\begin{itemize}
    \item Layer Integrated Gradients (\textbf{LIG}) settings: \\
    \# samples = 25.
    
    \item \textbf{LIME} settings: \\
    \# samples = 25; perturbation function = applying a [PAD] token mask with a masking probability = 0.3; token similarity kernel following \citet{atanasova-etal-2020-diagnostic}; interpretable model = linear least squares model with l2 regularization.
    
    \item Occlusion (\textbf{Occ}) settings: \\
    sliding window = 3.
    
    \item Shapley Value Sampling (\textbf{SVS}) settings: \\
    \# samples = 25.
\end{itemize}

\subsection*{GPU infrastructure}
\label{sec:gpu-infra}
To produce the feature attribution maps, we used up to 24 NVIDIA GPUs in parallel, namely GTX 1080Ti, RTX 2080Ti, RTX 3090, Quadro RTX 6000 and RTX A6000. 

\subsection*{Heatmap visualization}

We based our visualization of feature attribution maps on the displaCy visualizer which is part of the spaCy library \cite{spacy}. Specifically, we discovered a Jupyter notebook demo\footnote{\url{https://nbviewer.jupyter.org/github/galtay/displacy_token_heat/blob/master/token_heat.ipynb}} that made use of it and based our implementation on it.

In related works, we also found matplotlib-based visualizer implementations by \citet{Tsang2020HowDT}\footnote{\url{https://github.com/mtsang/archipelago/tree/main/src/viz}} and \citet{Bodria2021BenchmarkingAS}\footnote{\url{https://nbviewer.jupyter.org/github/kdd-lab/XAI-Survey/blob/main/Examples_Text.ipynb}} and considered the Ecco library by Alammar (2021)\footnote{\url{https://github.com/jalammar/ecco}} before eventually choosing the easier-to-handle displaCy.
